# Supplementary material for: Centralized and decentral approaches to succeed the 100% energiewende in Germany in the European context: A model-based analysis of generation, network, and storage investments
Source: arXiv:2205.09066 source file (2022-05-18)
Supplement: Supplementary file 1 [file appendix.tex]

\appendix
